# Supplementary material for: A unified and consistent electrical double layer model for treatment of core and space charge layer in solid electrolytes
Source: arXiv:2412.17750 source file (2024-12-23)
Supplement: Supplementary file 1 [file suppinfo.pdf]

# Supporting Information: A unified and consistent electrical double layer model for treatment of core and space charge layer in solid electrolytes

Zeeshan Ahmad*

*Department of Mechanical Engineering, Texas Tech University, Lubbock, Texas 79409, USA*

E-mail: zeeahmad@ttu.edu

# 1 Change of potential reference

The electrochemical potential of the defects is given by:

$$\mu_+(x) = \mu_+^{b0} - B_+ \exp\left(-\frac{x}{\lambda_{c+}}\right) + \frac{f_+ c_+^2}{(1-c_+)^2} + f_c c^- + z_+ e\phi + kT \ln\left(\frac{c_+}{1-c_+}\right) = 0 \quad \text{(1a)}$$

$$\mu_-(x) = \mu_-^{b0} - B_- \exp\left(-\frac{x}{\lambda_{c-}}\right) + \frac{f_- c_-^2}{(1-c_-)^2} + f_c c^+ - z_- e\phi + kT \ln\left(\frac{c_-}{1-c_-}\right) = 0 \quad \text{(1b)}$$

In the bulk ($x \to \infty$), the concentrations are low enough so that 1) $kT \ln[c/(1-c)] \to kT \ln(c)$ and 2) interactions are absent. The simplified equations are:

$$\mu_+(x) = \mu_+^{b0} + z_+ e\phi + kT \ln(c_+) = 0 \quad \text{(2a)}$$

$$\mu_-(x) = \mu_-^{b0} - z_- e\phi + kT \ln(c_-) = 0 \quad \text{(2b)}$$

Since bulk electroneutrality holds,[1] $N_+ z_+ c_+ = N_- z_- c_-$ and $c_- = N_+ z_+ c_+ / N_- z_-$ can be substituted in Eq. 2b

$$\mu_-(x) = \mu_-^{b0} - z_- e\phi + kT[\ln(c_+) + \ln(N_+ z_+ / N_- z_-)] = 0 \quad \text{(3)}$$

$$kT \ln(c_+) = -\mu_-^{b0} + z_- e\phi - kT \ln(N_+ z_+ / N_- z_-) \quad \text{(4)}$$

From this equation, the value of $kT \ln(c_+)$ can be substituted in Eq. 2a:

$$\mu_+(x) = \mu_+^{b0} + z_+ e\phi - \mu_-^{b0} + z_- e\phi - kT \ln(N_+ z_+ / N_- z_-) = 0 \quad \text{(5)}$$

This gives the potential in the bulk as:

$$\phi = \frac{\mu_-^{b0} - \mu_+^{b0} + kT \ln(N_+ z_+ / N_- z_-)}{e(z_+ + z_-)} \quad \text{(6)}$$

We change the reference such that the potential is zero in the bulk using the transforma-

tion:

$$\phi^{'} = \phi - \frac{\mu_-^{b0} - \mu_+^{b0} + kT\ln(N_+z_+/N_-z_-)}{e(z_+ + z_-)} \tag{7}$$

In this reference, Eq. 1 becomes:

$$\begin{aligned}
\mu_+(x) = \frac{\mu_+^{b0} + \mu_-^{b0}}{e(z_+ + z_-)} + \frac{kT}{e(z_+ + z_-)} \ln\left(\frac{N_+z_+}{N_-z_-}\right) - B_+ \exp\left(-\frac{x}{\lambda_{c+}}\right) + \frac{f_+c_+^2}{(1-c_+)^2} + f_c c^- \\
+z_+e\phi^{'} + kT\ln\left(\frac{c_+}{1-c_+}\right) = 0 \\
\mu_-(x) = \frac{\mu_+^{b0} + \mu_-^{b0}}{e(z_+ + z_-)} - \frac{kT}{e(z_+ + z_-)} \ln\left(\frac{N_+z_+}{N_-z_-}\right) - B_- \exp\left(-\frac{x}{\lambda_{c-}}\right) + \frac{f_-c_-^2}{(1-c_-)^2} + f_c c^+ \\
-z_-e\phi^{'} + kT\ln\left(\frac{c_-}{1-c_-}\right) = 0
\end{aligned} \tag{8}$$

# References


(1) Maier, J. Ionic Conduction in Space Charge Regions. *Progress in Solid State Chemistry* **1995**, *23*, 171–263.
